# Supplementary material for: A fast and strong microactuator powered by internal combustion of hydrogen and oxygen
Source: arXiv:2408.03103 source file (2024-08-06)
Supplement: Supplementary file 1 [file SI.pdf]

**Supplemental Information**

**Text S1. Details of the force evaluation**

To describe the motion of the ball under the influence of the actuator, one can use Newton's equation:

$$m\frac{d^2z}{dt^2} = F(t) \tag{1}$$

where $m$ is the mass of the ball and $z$ is the coordinate of its center. The force $F(t)$ is acting on the ball at a given time $t$. The actuator applies the force to the ball for a short time, $t_0$, much shorter than the time it takes for the ball to reach its highest point on the trajectory. In the interval $0 < t < t_0$, the force changes fast with time, but, for simplicity, one can consider it as a constant equal to an average value in this interval. Let us define this average force as

$$F_0 = \frac{1}{t_0}\int_0^{t_0} F(t)dt = ma \tag{2}$$

where an acceleration $a$ is defined by the relation (2). When the ball loses contact with the membrane of the actuator, only the gravity force acts on the ball, which is equal to $-mg$ where $g$ is the free-fall acceleration. Thus, Eq. (1) can be rewritten in the following form:

$$\frac{d^2z}{dt^2} = \begin{cases} a, & t < t_0 \\ -g, & t \geq t_{0.} \end{cases} \tag{3}$$

In the initial moment $t = 0$ both the position and velocity of the ball are zero. Since the ball trajectory is observed at $t \gg t_0$, the role of the initial interval is just to give some velocity to the body that can be considered as an initial velocity for the free movement of the ball. This initial velocity is $v_0 = at_0$ and the initial position is $z_0 = at_0^2/2$. The latter value is less than the stroke of the unloaded membrane, which is about 100 μm and can be neglected on a length scale of 10 mm. Thus, the solution of Eq. (3) at $t \geq t_0$ is

$$z(t) \approx -\frac{1}{2}gt^2 + v_0 t. \tag{4}$$

From this relationship, one finds the highest point of the trajectory $H = v_0^2/2g$ and the moment when this point is reached $t_f = v_0/g$. Measuring experimentally the value of $H$, one finds the unknown initial velocity and rising time

$$v_0 = \sqrt{2gH}, \;\; t_f = \sqrt{2H/g}. \tag{5}$$

These relations have been used in the main text. The instantaneous force acting on the body is then determined from Eq. (2) as

$$F_0 = mv_0/t_0. \tag{6}$$

Here the time $t_0 \approx 10\,\mu s$ is determined from the observation of the current behavior during the explosion. Note that this time does not change in dependence on the load.

**Fig. S1. Current and position of the frames from Movie S1**

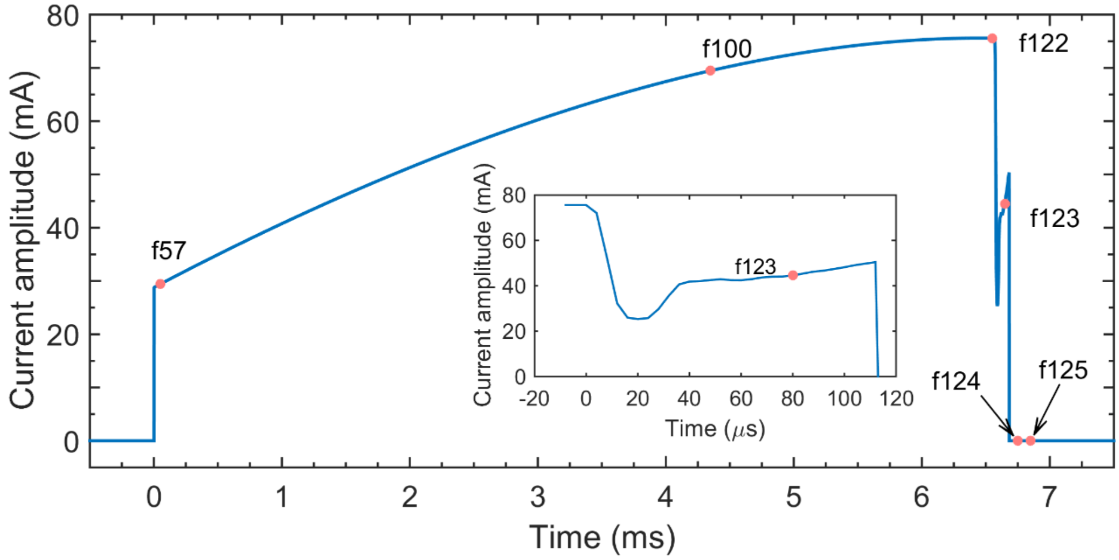


**Figure S1.** The current amplitude that corresponds to Movie S1. The positions of the frames shown in Fig. 2A are indicated by red circles. The current starts to drop due to the formation of an exploding bubble at the moment $t = 6.570$ ms. This time is taken as the initial moment in the inset that shows the current during the explosion in detail.

**Fig. S2. Comparison of the currents near explosion for unloaded and loaded cases**

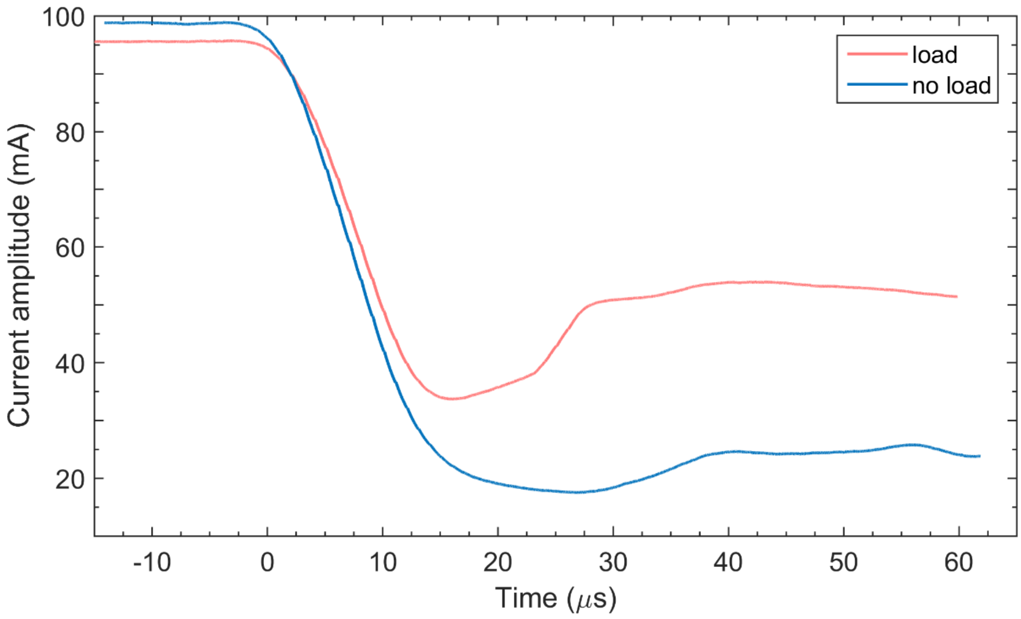


**Figure S2.** Current amplitude near the explosion averaged over two periods (4 μs). The initial moment is taken at the beginning of the explosion. The rate of current decrease (increase of the bubble) is similar, but for the unloaded case, the bubble grows larger and keeps its larger size longer than for the loaded case.

**Fig. S3. Sequence of the fabrication steps**

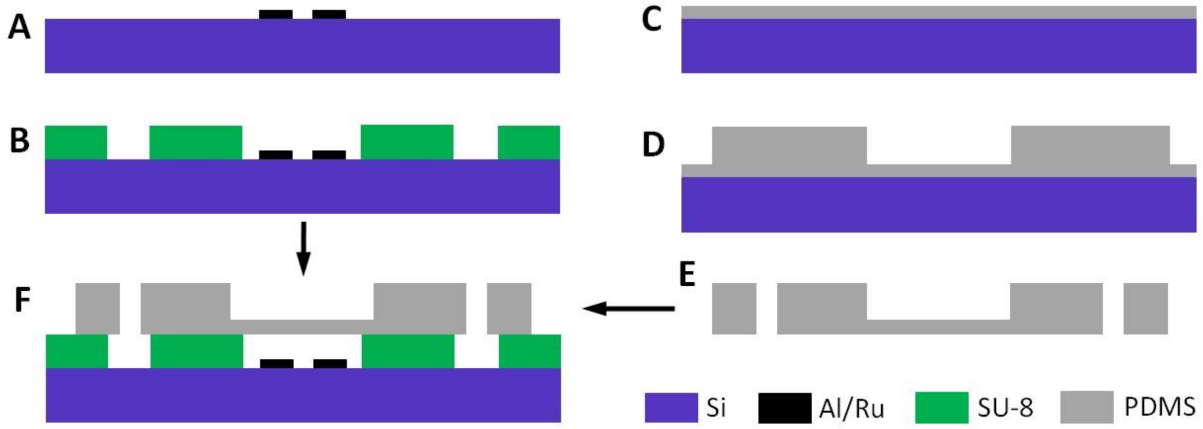


**Figure S3.** Fabrication of the actuator. (**A**) Patterning the electrodes. (**B**) Formation of the chamber and channels. (**C**) Formation of the membrane layer. (**D**) Bonding of a thick PDMS block to the membrane layer. (**E**) Detachment of PDMS from the substrate and punching the holes. (**F**) Bonding of PDMS to SU-8.

**Fig. S4. Scheme of the experiment**

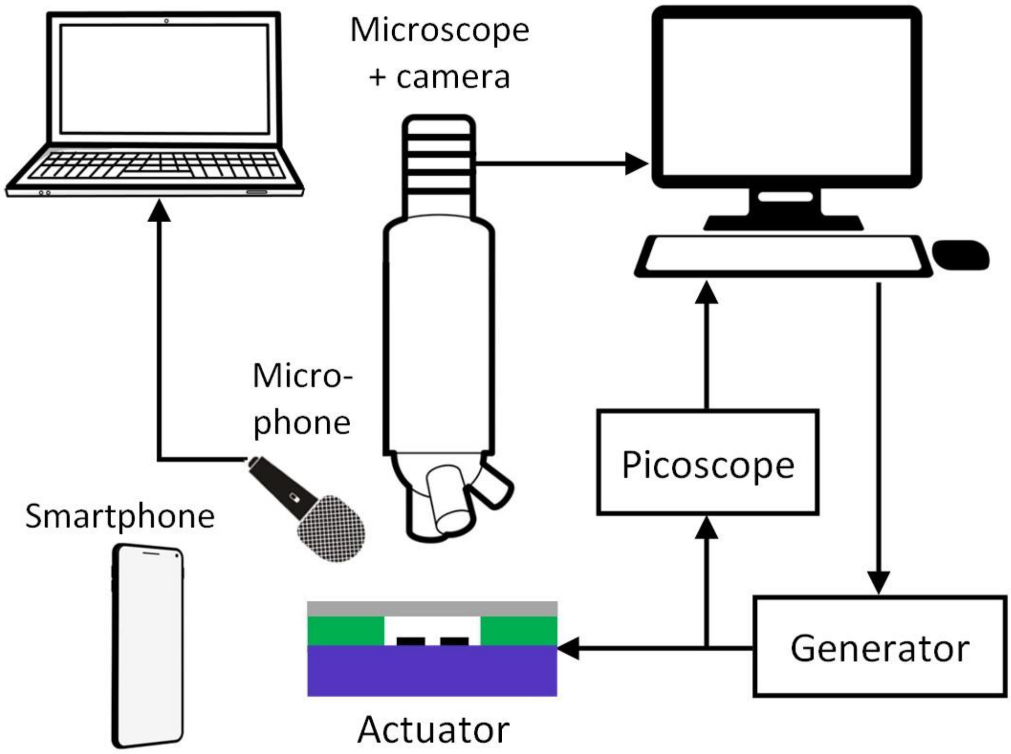


**Figure S4.** Scheme of the experiment showing the elements used for characterization.

**Fig. S5. Testing platform**

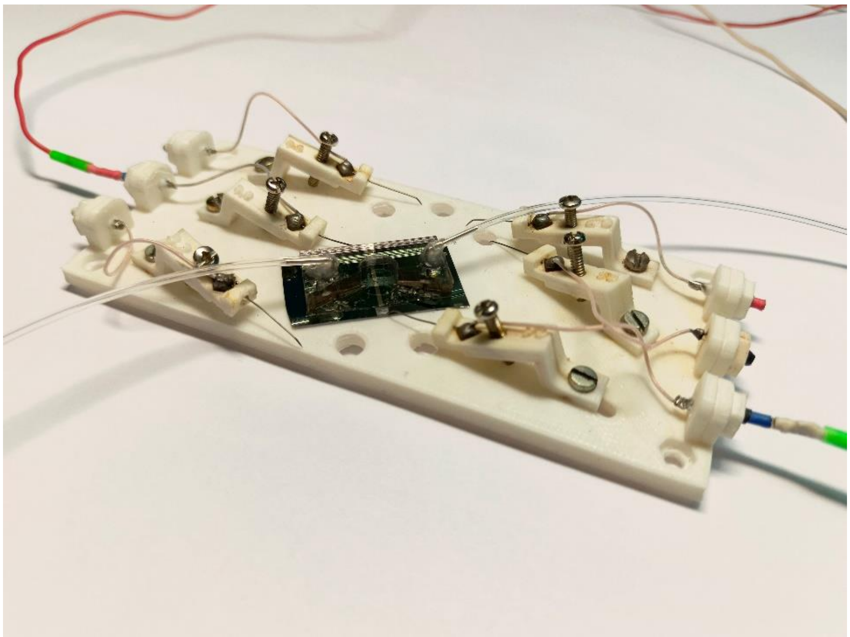

**Figure S5.** 3D-printed platform used for characterization of the actuator.

**Table S1. Chemical composition of electrodes after 40,000 explosions**

| Element and line | C K | O K | Na K | Al K | Si K | S K | Ru L |
|---|---|---|---|---|---|---|---|
| Content of element in point 1, at% | 1.75 | 16.81 | 0.64 | 0.98 | 1.75 | 0.99 | 77.08 |
| Content of element in point 2, at% | 8.15 | 25.90 | 0.69 | 1.65 | 2.86 | 1.09 | 59.66 |

**Table S1.** Chemical composition was determined using an energy-dispersive X-ray spectrometer at an accelerating voltage of 6 kV. The main elements present are Ru and O. A significant amount of oxygen indicates oxidation of ruthenium, but it does not influence the performance of the actuator. The amount of oxygen is higher at the edge of the central electrode. Some amount of carbon can arise from PDMS and SU-8.
